# Supplementary material for: Dual topological superconducting states in the layered titanium-based oxypnictide superconductor BaTi$_2$Sb$_2$O
Source: arXiv:2009.06805 source file (2020-09-15)
Supplement: Supplementary file 1 [file SM.pdf]

# Supplemental Material for Dual topological superconducting states in the titanium-based oxypnictide superconductor $BaTi_2Sb_2O$

Z. Huang,[1,2,3,*] W. L. Liu,[1,2,3,*] H. Y. Wang,[3,*] Y. L. Su,[3,*] Z. T. Liu,[1,*] X. B. Shi,[4,5] S. Y. Gao,[6] Z. C. Jiang,[1] Z. H. Liu,[1] J. S. Liu,[1] X. L. Lu,[1] Y. C. Yang,[1] J. X. Zhang,[3,7] S. C. Huan,[3] W. Xia,[3,8] J. H. Wang,[3,8] Y. S. Wu,[3] X. Wang,[3,9] N. Yu,[3,9] Y. B. Huang,[10] S. Qiao,[1] J. Li,[3,8] W. W. Zhao,[4,5] Y. F. Guo,[3,†] G. Li,[3,8,‡] and D. W. Shen[1,2,§]

[1]*Center for Excellence in Superconducting Electronics,*
*State Key Laboratory of Functional Materials for Informatics,*
*Shanghai Institute of Microsystem and Information Technology,*
*Chinese Academy of Sciences, Shanghai 200050, China*

[2]*Center of Materials Science and Optoelectronics Engineering,*
*University of Chinese Academy of Sciences, Beijing 100049, China*

[3]*School of Physical Science and Technology, ShanghaiTech University, Shanghai 201210, China*

[4]*State Key Laboratory of Advanced Welding and Joining,*
*Harbin Institute of Technology, Shenzhen 518055, China*

[5]*Flexible Printed Electronics Technology Center, Harbin Institute of Technology, Shenzhen 518055, China*

[6]*Beijing National Laboratory for Condensed Matter Physics and Institute of Physics, Chinese Academy of Sciences, Beijing 100190, China*

[7]*Institute for Advanced Study, Tsinghua University, Beijing 100084, China*

[8]*ShanghaiTech Laboratory for Topological Physics, ShanghaiTech University, Shanghai 201210, China*

[9]*Analytical Instrumentation Center, School of Physical Science and Technology, ShanghaiTech University, Shanghai 201210, China*

[10]*Shanghai Synchrotron Radiation Facility, Shanghai Advanced Research Institute,*
*Chinese Academy of Sciences, 201204 Shanghai, China*

## I. SUPPLEMENTARY NOTE 1: DETAILS ON THE SAMPLE GROWTH METHOD AND CHARACTERIZATIONS

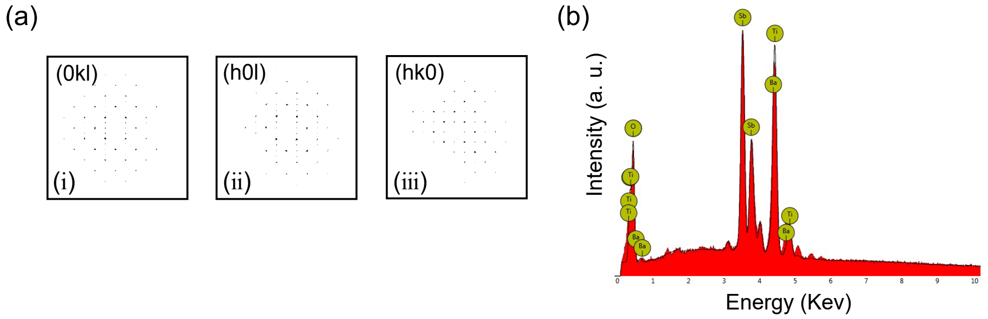


FIG. S1. (a) (*i*)-(*iii*) are X-ray diffraction patterns from the (0kl), (h0l) and (hk0) surfaces. (b) The energy dispersive X-ray spectrometry (EDS) intensity of $BaTi_2Sb_2O$.

High-quality single crystals of $BaTi_2Sb_2O$ were grown by using $BaSb_2$ as the flux. Pieces of Ba (99.95%), Sb (99.999%) and TiO (99.9%) were mixed with an atomic ratio of Ba : Sb : TiO = 10 : 20 : 1, and then placed in an alumina crucible. This crucible was later sealed into a tantalum tube, which was then sealed into a quartz tube. The assembly was heated up to 1100°C, maintained more than 30 hours, and was then slowly cooled down to 900°C at a temperature decreasing rate of 2°C/h. At 580°C the flux was immediately separated in a high speed centrifuge. $BaTi_2Sb_2O$ single crystals were thus obtained in the aluminium oxide crucible.

Then they have been further characterized by the single-crystal XRD [Fig.S1(a)], through which the space group P/4mmm (no. 123) can be verified with lattice constants $a = b = 4.1063$ Å and $c = 8.0641$ Å, in good agreement with previous reports[1]. The energy dispersive X-ray spectrometer (EDS) result demonstrates the elements composition of this compound, which exhibits the Ba, Ti, Sb and O peaks [Fig.S1(b)].

## II. SUPPLEMENTARY NOTE 2: DETAILS ON THE CALCULATION

First-principles calculations were performed within the framework of the projector augmented wave (PAW)[2] method and selected the generalized gradient approximation (GGA)[3] with Perdew-Burke-Ernzerhof (PBE) type[4], as encoded in the Vienna Ab initio Simulation Package (VASP)[5]. A kinetic energy cutoff of 500 eV, a Γ-centred k mesh of $12 \times 12 \times 6$, and an energy difference criterion $10^{-6}$ eV were utilized for all calculations. The spin-orbit coupling (SOC) was considered in a self-consistent manner. The WANNIER90 package[6] was adopted to construct Wannier functions from the first-principles results. Topological properties calculations were carried out with our in-house code *TMC*.

## III. SUPPLEMENTARY NOTE 3: DETAILS ON THE ARPES EXPERIMENT

High-resolution and spin-resolved ARPES measurements were performed at 03U and "Dreamline" beam lines of Shanghai Synchrotron Radiation Facility (SSRF), respectively. The 03U endstation is equipped with a Scienta Omicron DA30 electron analyzer. All ARPES data were taken at 15 K in an ultrahigh vacuum better than $8.0 \times 10^{-11}$ Torr. The angular and the energy resolutions were set to 0.2° and 6~20 meV (dependent on the selected probing photon energy), respectively. The spin-resolved ARPES at "Dreamline" is equipped with a Scienta Omicron DA30-L electron analyzer together with a spin detector based on the very-low-energy-electron-diffraction (VLEED).

## IV. SUPPLEMENTARY NOTE 4: $k \cdot p$ MODEL FOR THE DP AND THE GAP ALONG $\Gamma$-$Z$

The bulk DP along $\Gamma$-$Z$ is symmetry protected, i.e., as long as two bands cross, their crossing point will be stable against symmetry-allowed perturbations. For arbitrary $k_z$ point between $\Gamma$ and $Z$, the little group contains $\hat{c}_{2z}$ and $\hat{c}_4$. In addition, the joint operation of the anti-unitary $\hat{\mathcal{T}}$ with other three crystalline symmetries, i.e., $\hat{c}_{2y}$, $\hat{c}_{2x}$, and $\hat{\mathcal{I}}$ will also leave $k_z$ invariant. With these symmetry constrains, we can write down a $k \cdot p$ model to resolve both the symmetry-protected DP and the unavoidable gap below. It should be noted that it is sufficient for $\hat{\mathcal{T}}\hat{\mathcal{I}}$ and $\hat{c}_4$ to protect a DP. The inclusion of the other symmetries helps to further simplify the model.

The basis functions of $\Gamma_6^-$, $\Gamma_7^-$, and $\Gamma_7^+$ are $|\frac{1}{2}, \frac{1}{2}\rangle^\bullet$, $|\frac{1}{2}, -\frac{1}{2}\rangle^\bullet$, $|\frac{3}{2}, -\frac{3}{2}\rangle^\bullet$, $|\frac{3}{2}, \frac{3}{2}\rangle^\bullet$, $|\frac{3}{2}, -\frac{3}{2}\rangle$, and $|\frac{3}{2}, \frac{3}{2}\rangle$. Here $|J, mj\rangle^{(\bullet)}$ is the relativistic basis function, and the symbol $\bullet$ on the shoulder denoting its anti-symmetric(symmetric) response to $\hat{\mathcal{I}}$. Under these basis functions, it is straightforward to obtain the representation matrix for $\hat{c}_2$, $\hat{c}_4$, $\hat{\mathcal{T}}\hat{\mathcal{I}}$, $\hat{\mathcal{T}}\hat{c}_{2x}$, and $\hat{\mathcal{T}}\hat{c}_{2y}$, which can be compactly written as $\hat{c}_{2z} = -i\tau_0^3\sigma_z$, $\hat{c}_{4z} = \tau_1^3\sigma_\epsilon$, $\hat{\mathcal{T}}\hat{\mathcal{I}} = i\tau_2^3\sigma_y\mathcal{K}$, $\hat{\mathcal{T}}\hat{c}_{2x} = -i\tau_0^3\sigma_z\mathcal{K}$, and $\hat{\mathcal{T}}\hat{c}_{2y} = \tau_0^3\sigma_z\mathcal{K}$, where $\tau_{0-2}^3$ are $3 \times 3$ matrices with only diagonal elements $(1, 1, 1)$, $(1, -1, -1)$, and $(1, 1, -1)$, respectively. $\sigma_\epsilon$ is a $2 \times 2$ matrix with diagonal element $(\epsilon^*, \epsilon)$ and $\epsilon = \exp(i\pi/4)$.

$$\hat{c}_{2z} = \begin{pmatrix} -i & 0 & 0 & 0 & 0 & 0 \\ 0 & i & 0 & 0 & 0 & 0 \\ 0 & 0 & -i & 0 & 0 & 0 \\ 0 & 0 & 0 & i & 0 & 0 \\ 0 & 0 & 0 & 0 & -i & 0 \\ 0 & 0 & 0 & 0 & 0 & i \end{pmatrix}, \hat{c}_{4z} = \begin{pmatrix} \epsilon^* & 0 & 0 & 0 & 0 & 0 \\ 0 & \epsilon & 0 & 0 & 0 & 0 \\ 0 & 0 & -\epsilon^* & 0 & 0 & 0 \\ 0 & 0 & 0 & -\epsilon & 0 & 0 \\ 0 & 0 & 0 & 0 & -\epsilon^* & 0 \\ 0 & 0 & 0 & 0 & 0 & -\epsilon \end{pmatrix}. \quad (1)$$

$$\hat{\mathcal{T}}\hat{\mathcal{I}} = \begin{pmatrix} 0 & 1 & 0 & 0 & 0 & 0 \\ -1 & 0 & 0 & 0 & 0 & 0 \\ 0 & 0 & 0 & 1 & 0 & 0 \\ 0 & 0 & -1 & 0 & 0 & 0 \\ 0 & 0 & 0 & 0 & 0 & -1 \\ 0 & 0 & 0 & 0 & 1 & 0 \end{pmatrix} \mathcal{K}, \hat{\mathcal{T}}\hat{c}_{2x} = \begin{pmatrix} -i & 0 & 0 & 0 & 0 & 0 \\ 0 & i & 0 & 0 & 0 & 0 \\ 0 & 0 & -i & 0 & 0 & 0 \\ 0 & 0 & 0 & i & 0 & 0 \\ 0 & 0 & 0 & 0 & -i & 0 \\ 0 & 0 & 0 & 0 & 0 & i \end{pmatrix} \mathcal{K}, \hat{\mathcal{T}}\hat{c}_{2y} = \begin{pmatrix} 1 & 0 & 0 & 0 & 0 & 0 \\ 0 & -1 & 0 & 0 & 0 & 0 \\ 0 & 0 & 1 & 0 & 0 & 0 \\ 0 & 0 & 0 & -1 & 0 & 0 \\ 0 & 0 & 0 & 0 & 1 & 0 \\ 0 & 0 & 0 & 0 & 0 & -1 \end{pmatrix} \mathcal{K}.$$

The effective continuum model along $\Gamma$-$Z$ has the following form

$$H_z(k) = \begin{pmatrix} \mathcal{A}_1(k) & 0 & 0 & 0 & 0 & 0 \\ 0 & \mathcal{A}_1(k) & 0 & 0 & 0 & 0 \\ 0 & 0 & \mathcal{A}_2(k) & 0 & \mathcal{A}_4(k) & 0 \\ 0 & 0 & 0 & \mathcal{A}_2(k) & 0 & -\mathcal{A}_4(k) \\ 0 & 0 & \mathcal{A}_4^*(k) & 0 & \mathcal{A}_3(k) & 0 \\ 0 & 0 & 0 & -\mathcal{A}_4^*(k) & 0 & \mathcal{A}_3(k) \end{pmatrix} \quad (2)$$

with $\mathcal{A}_1(k) = a_1 + a_2k_z^2$, $\mathcal{A}_2(k) = a_3 + a_4k_z^2$, $\mathcal{A}_3(k) = a_5 + a_6k_z^2$, $\mathcal{A}_4(k) = a_7 + ia_8k_z + a_9k_z^2 + ia_{10}k_z^3$ with $a_1 \cdots a_{10}$ the parameters determined from fitting to the DFT band structure as $a_1 = 0.1478$ eV·Å$^2$, $a_2 = -2.5952$ eV·Å$^2$, $a_3 = 0.009$ eV·Å$^2$, $a_4 = -0.2538$ eV·Å$^2$, $a_5 = 0.0383$ eV·Å$^2$, $a_6 = -0.8993$ eV·Å$^2$, $a_7 = -0.1381$ eV·Å$^2$, $a_8 = 0.0501$ eV·Å$^2$, and $a_9 = 3.5192$ eV·Å$^2$. As clearly indicated by the model, there is no coupling between $\Gamma_6^-$ with either $\Gamma_7^-$ or $\Gamma_7^+$ states. Thus, the crossing of $\Gamma_6^-$ with any of the other two bands will always be stable and symmetry-protected, which leads to the DP. However, the coupling between $\Gamma_7^+$ and $\Gamma_7^-$ will gap any crossing between them explaining the small gap below the DP shown in Fig. 1(f) in the main text.

One can also understand the lift of the band degeneracy away from the DP in this model. The DP requires the protection of $\hat{c}_4$, which is not a symmetry for arbitrary $k$. As long as $k$ goes away $\Gamma$-$Z$, new Hamiltonian matrix elements appear which will ultimately remove the degeneracy of the DP. Thus, the DP shown in Fig. 1(f) in the main text is an anisotropic DP linear only along $\Gamma$-$Z$ direction. The additional Hamiltonian elements are found to be

$$H_{xy}(k) = \begin{pmatrix} \mathcal{B}_1(k) & 0 & \mathcal{B}_4(k) & 0 & \mathcal{B}_5(k) & 0 \\ 0 & \mathcal{B}_1(k) & 0 & \mathcal{B}_4(k) & 0 & -\mathcal{B}_5(k) \\ \mathcal{B}_4^*(k) & 0 & \mathcal{B}_2(k) & 0 & \mathcal{B}_6(k) & 0 \\ 0 & \mathcal{B}_4^*(k) & 0 & \mathcal{B}_2(k) & 0 & -\mathcal{B}_6(k) \\ \mathcal{B}_5^*(k) & 0 & \mathcal{B}_6^*(k) & 0 & \mathcal{B}_3(k) & 0 \\ 0 & -\mathcal{B}_5^*(k) & 0 & -\mathcal{B}_6^*(k) & 0 & \mathcal{B}_3(k) \end{pmatrix}, \quad (3)$$

with $\mathcal{B}_1(k) = b_1k_+^2$, $\mathcal{B}_2(k) = b_2k_+^2$, $\mathcal{B}_3(k) = b_3k_+^2$, $\mathcal{B}_4(k) = b_4k_-^2 + b_5k_xk_y + b_6ik_-^2k_z + ib_7k_xk_yk_z$, $\mathcal{B}_5(k) = b_8k_-^2 + b_9k_xk_y + ib_{10}k_-^2k_z + ib_{11}k_xk_yk_z$, $\mathcal{B}_6(k) = b_{12}k_+^2 + ib_{13}k_+^2k_z$, and $k_\pm^2 = k_x^2 \pm k_y^2$. It is clear that All three bands couple together. Consequently, no stable band degeneracy is guaranteed whenever $k$ is away from $\Gamma$-$Z$.

## V. SUPPLEMENTARY NOTE 5: EXPERIMENT GEOMETRY OF THE ARPES MEASUREMENT

Under the foundation of the three-step model and sudden approximation[7], the intensity measured in ARPES experiment I(**k**, E),

$$I(\mathbf{k}, E) = I_0(\mathbf{k}, v, \mathbf{A})A(\mathbf{k}, E)f(E, T) \tag{4}$$

where the matrix term on the right-hand $\mathrm{I}_0(\mathbf{k}, \mathrm{v}, \mathbf{A}) \propto \sum_{f,i}|\mathrm{M}_{f,i}^k|^2$, and the photoemission matrix element $\mathrm{M}_{f,i}^k = \phi_f^k|\mathbf{A}\cdot\mathbf{p}|\phi_i^k$. This term describe the wavefunction transition from the initial states $\phi_i^k$ to the final states $\phi_f^k$. The photon polarization and energy dependent vector potential **A** and position operator **p** also affect the measured results. Therefore, the photon configuration and measurement geometries modulate the measured ARPES intensity of initial states with different symmetries.

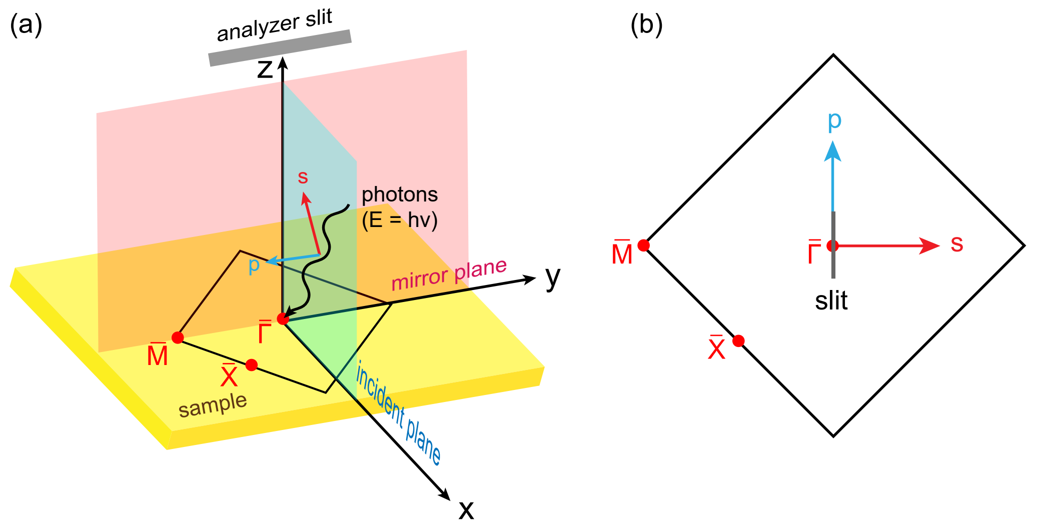


FIG. S2. (a) The experimental polarization setup for our experiment. The incident plane is normal to the analyzer slit and the sample plane. The mirror plane is normal to the sample plane and parallel to the analyzer slit. The electric field of $p$-polarized photons are within the mirror plane with $y$ direction polarization component, and the $s$-polarized photons are perpendicular to the mirror plane with $x$ and $z$ direction polarization component. (b) The measurement geometry in the (001) surface Brillouin Zone for our sample.

The data showing in the main text were collected by utilizing linear horizontal ($s$ geometry) [Fig. 3] and vertical ($p$ geometry) [Fig. 2] photons at 03U and Dreamline beamlines of Shanghai Synchrotron Radiation Facility (SSRF). These beamlines are equipped with the same measurement geometry as shown in Fig. S2 with $p$-polarized photons parallel to the measured $\bar{\Gamma}$-$\bar{M}$

direction and $s$-polarized photons vertical to the measured direction. It is helpful to use different measurement geometry and photon energy to distinguish the surface states and bulk states in our sample as discussed below.

We displayed the intensity maps of $k_z$-$k_m$ plane under $p$-polarized photons [Fig S3(a)] and $s$-polarized photons [Fig S3(b)] and corresponding second derivative plots in the main text [Fig. 2(b) and Fig. 3(b)]. Under the measurement with wide range of photon energies, there are negligible $k_z$ dispersions by using $s$-polarized photons [Fig S3(b)], while the periodic modulation along $k_z$ direction by $p$-polarized photons can be recognized [Fig S3(a)]. Note that because of the longer inelastic mean free path of excited photoelectrons under larger photon energies, the periodic modulation of bulk states is much more clear under photon energies above 80 eV. Consequently, we separate the surface states and bulk states using polarization dependent measurement. The $s$ geometry is sensitive to the $k_z$ independent surface states. The $p$ geometry is beneficial to detect the $k_z$ dependent bulk states.

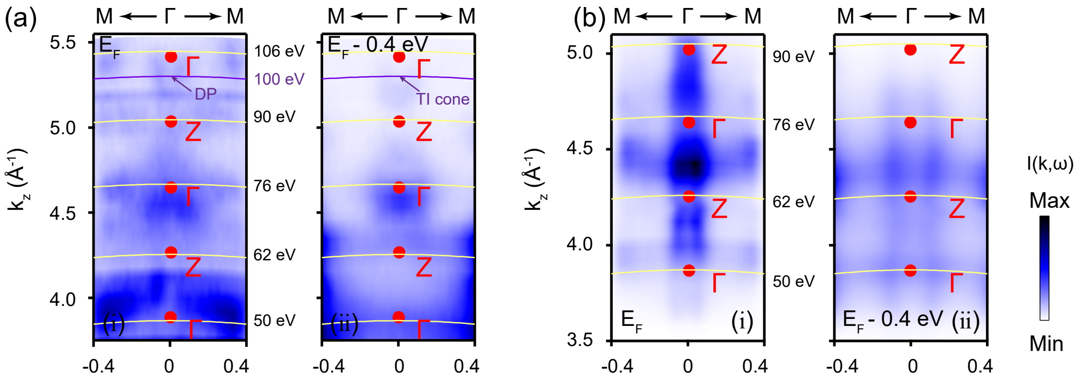


FIG. S3. (a) Intensity plot of $k_z$ dependent ARPES data along $\Gamma$-$M$ direction with $p$-polarized photons at $E_F$ ($i$) and $E_F$ - 0.4 eV ($ii$), respectively. The photon energies used for $k_z$ dispersion measurement are from 46 to 110 eV. (b) Intensity plot of $k_z$ dependent ARPES data along $\Gamma$-$M$ direction with $s$-polarized photons at $E_F$ ($i$) and $E_F$ - 0.4 eV ($ii$), respectively. The photon energies used for $k_z$ dispersion measurement are from 40 to 94 eV.

## VI. SUPPLEMENTARY NOTE 6: PHOTON ENERGY DEPENDENCE OF THE ARPES MEASUREMENT

Here, we discuss the $k_z$-momentum determination. Since the surface of the measured sample breaks the translational symmetry along out-of-plane direction, the perpendicular momentum components of the photonelectron ($k_\perp^f$) and the initial electron ($k_\perp^i$) are not equivalent. Although we can not get the out-of-plane momentum directly as the in-plane momentum ($k_x$, $k_y$ and $k_m$), it is helpful to determine the $k_z$ momentum based on the nearly free-electron approximation for final states[8],

$$k_\perp^{\mathrm{i}} = \sqrt{2m(E_{\mathrm{kin}} \cos^2\theta) + V_0}/\hbar \tag{5}$$

where $V_0$ is the inner potential which is a constant and can be defined by fitting the periodicity of different photon energy measurement. Through a wide range of photon energy dependent ARPES measurement (from 46 to 110 eV in Fig. S3(a)), we get the inner potential $V_0 = 11$ eV in $BaTi_2Sb_2O$. Thus, we can determine the exact value of $k_\perp$ and corresponding high symmetry points.

The intensity map of $k_z$-$k_m$ plane at $E_F$ indicates the evolution of BB1, which is the upper part of TDS states. When BB1 becomes broadest under 100 eV photons, it intersects through the TDS cone. The intensity map of $k_z$-$k_m$ plane at $E_F$ - 0.4 eV indicates the evolution of BB2, which is the lower part of TI states. When BB2 becomes broadest under 100 eV photons, it intersects through the TI cone. These two topological states are close along $k_z$ direction as the calculated result in Fig. 1(f) in the main text and is detectable under 100 eV photons.

## VII. SUPPLEMENTARY NOTE 7: CONSTANT-ENERGY SURFACE SPIN TEXTURE CALCULATIONS

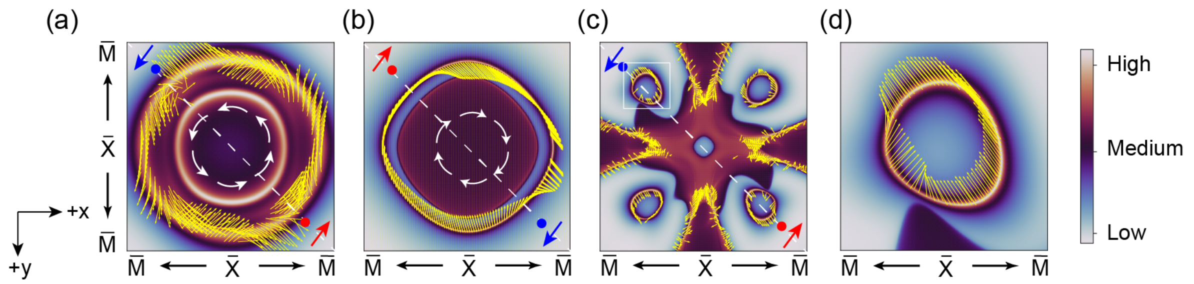


FIG. S4. (a)-(c) Calculated spin textures at $E_B$ = -0.02 eV, -0.12 eV and -0.3 eV, where their helical natures of SS1, SS2 and SS3 are clearly visible. (d) A zoom-in plot for the region shown as the white box in (c).

To further confirm the helical nature of the three surface bands (SS1 to SS3) in Fig. 4 (a) in the main text, we show the constant-energy plots of the surface states at three different energies, corresponding precisely to the energy levels measured in the experiment. On top of each plot, the spin moments $\langle S_x \rangle$ and $\langle S_y \rangle$ are plotted as vector field. The binding energy of Fig. S4(a) and (b) are $E_B$ = -0.02 eV and -0.12 eV, respectively. The helicity of the lower part of TI states (SS2) is obvious, while that for the upper part of TDS states (SS1) is slightly disturbed by the hybridization with the bulk bands. We note that we performed the calculation along $(00\bar{1})$ direction. Therefore, both the TDS and TI cones are of left-hand helicity and consistent with most TIs.

In contrast, at $E_B = -0.3$ eV, the lower surface Dirac bands are too far away from the surface DP, and they do not form a closed cone anymore. We instead observed four small closed surface loops with uniform spin orientations in each. The pocket in the top left corner of Fig. S4(c) are enlarged in Fig. S4(d) for better visualization. The spin texture of SS1 to SS3 is summarized in Fig. 4(b).

## VIII. SUPPLEMENTARY NOTE 8: DETAILS ON THE SPIN-RESOLVED ARPES MEASUREMENT

For the sake of extracting the unknown spin polarization $P$, we should measure the two spin intensity from opposite direction. The spin-detector we used distinguishes the spin polarized electrons along +$\hat{y}$ and -$\hat{y}$, thus we get the measured raw intensities $I_y^+$ and $I_y^-$. Since the measurement asymmetry, we can get the asymmetry,

$$A = \frac{I_y^+ - I_y^-}{I_y^+ + I_y^-} \tag{6}$$

the spin-polarization of the electron beam $P$,

$$P = \frac{A}{S} \tag{7}$$

where $S$ is the effective Sherman function of the spin detector. It corresponds to the asymmetry of a fully polarized electron beam. For our working situation at 6.3 ± 0.1 eV scattering energy, the Sherman function we used is $S$ = 0.275 ± 0.01 for the measured with a double scattering measurement.

Thus, the partial intensities,

$$N_\pm = \frac{I_{\text{tol}}}{2}(1 \pm P) \tag{8}$$

where $I_{tol} = I_y^+ + I_y^-$. The spin difference D, D = $N_y^+$ - $N_y^-$ and the raw difference D$_r$, D$_r$ = $I_y^+$ - $I_y^-$.

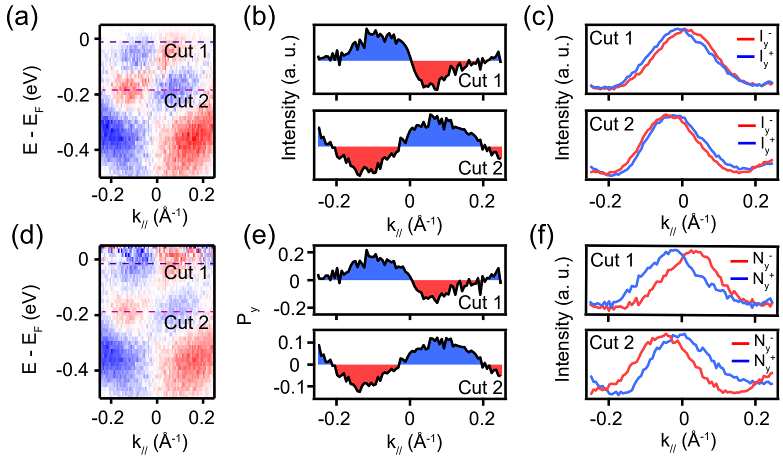


FIG. S5. (a) Spin difference intensity plots along the $\bar{\Gamma}$-$\bar{M}$ direction. (b) MDCs of (a) at $E_B$ = -0.03 eV and -0.18 eV marked as Cut 1 and 2. (c) raw spin intensity from +$\hat{y}$ and -$\hat{y}$ at Cut 1 and 2. (d) Spin polarization intensity plots along the $\bar{\Gamma}$-$\bar{M}$ direction. (e) MDCs of (d) at $E_B$ = -0.03 eV and -0.18 eV marked as Cut 1 and 2. (f) partial spin intensity from +$\hat{y}$ and -$\hat{y}$ at Cut 1 and 2.

The above spin difference and spin polarization image are shown in Fig. S5(a) and (d). MDCs of the two surface states SS1 and SS2 from TDS and TI states are also displayed. The partial intensity plots peaks in Fig. S5(f) indicate the exact momentum of surface band SS1 and SS2.

## IX. SUPPLEMENTARY NOTE 9: ARPES MEASUREMENT FOR CARRIER DOPING $BATI_2SB_2O$

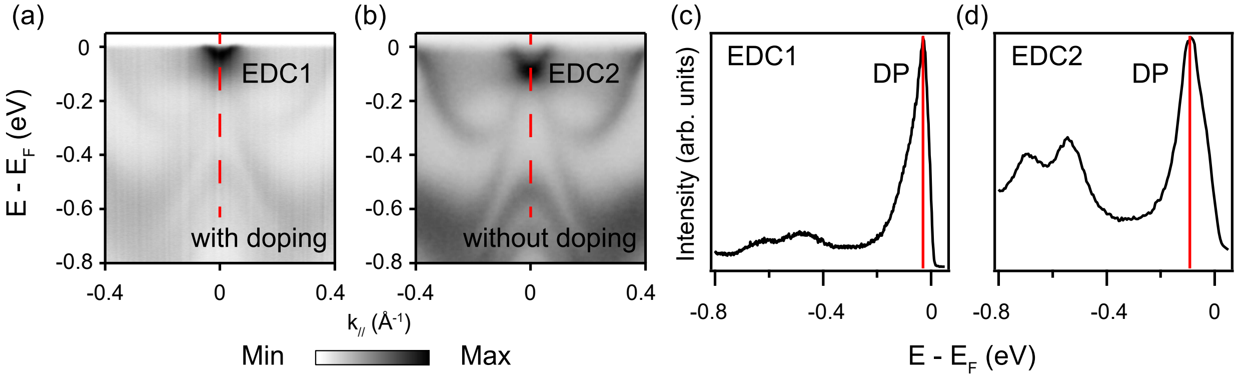


FIG. S6. (a) Intensity plot along $\bar{\Gamma}$-$\bar{M}$ direction with Na doping. (b) Intensity plot along $\bar{\Gamma}$-$\bar{M}$ direction without Na doping. (c) The momentum distribution curves (EDCs) of (a) with DP peak marked. (d) EDCs of (b) with DP peak marked.

The Intensity plot along $\bar{\Gamma}$-$\bar{M}$ direction with Na doping is shown in Fig. S6(a). Compared to the result without doping in Fig. S6(b), the Fermi level is explicit tuned lower. Further EDCs in Fig. S6(c) and (d) demonstrate the tunable Fermi level quantitatively.

---

* Equal contributions

† guoyf@shanghaitech.edu.cn

‡ ligang@shanghaitech.edu.cn

§ dwshen@mail.sim.ac.cn

[1] Yajima T et al, J. Phys. Soc. **81**, 10 (2012).

[2] Lehtomki J et al, J. Chem. Phys. **141**, 234102 (2014).

[3] Perdew J P et al, Phys. Rev. B **45**, 13244 (1992).

[4] Perdew J P et al, Phys. Rev. Lett. **77**, 3865 (1996).

[5] Kresse G et al, Phys. Rev. B **47**, 558 (1993).

[6] Mostofi A A et al, Comput. Phys. Commun. **178**, 685 (2008).

[7] Damascelli A et al, Rev. Mod. Phys. **75**, 473 (2003).

[8] Lv B et al, Nat. Rev. Phys. **1**, 609-626 (2019).
